# Supplementary material for: A topological criterion for filtering information in complex brain networks
Source: arXiv:1603.08445 source file (2016-11-23)
Supplement: Supplementary file 1 [file Supplementary_Information.tex]

%\documentclass[fleqn,12pt]{wlscirep}
%
%\usepackage{color}
%\usepackage{ulem}
%\usepackage{soul}
%\usepackage{multirow}
%\usepackage{array}
%\usepackage{amsmath}
%\usepackage{amsfonts}
%\usepackage{amssymb}
%%\usepackage{rotating}
%%\usepackage{pdflscape}
%%\usepackage{booktabs}
%\usepackage{caption}
%\captionsetup{justification=justified}
%\usepackage{xr}
%%\usepackage{hyperref}
%\externaldocument{Manuscript}
%%
%
%
%\usepackage{float}
%\DeclareMathAlphabet{\mathpzc}{OT1}{pzc}{m}{it}
%\usepackage{lineno}
%%\linenumbers
%
%
%\newcolumntype{L}[1]{>{\raggedright\let\newline\\\arraybackslash\hspace{0pt}}m{#1}}
%\newcolumntype{C}[1]{>{\centering\let\newline\\\arraybackslash\hspace{0pt}}m{#1}}
%\newcolumntype{R}[1]{>{\raggedleft\let\newline\\\arraybackslash\hspace{0pt}}m{#1}}
%
%\makeatletter
%\DeclareRobustCommand*\textsubscript[1]{%
%  \@textsubscript{\selectfont#1}}
%\def\@textsubscript#1{%
%  {\m@th\ensuremath{_{\mbox{\fontsize\sf@size\z@#1}}}}}
%\makeatother
%
%
%\begin{document}

%%% FIGURES AND TABLES

\section*{Supplementary Figures}

\begin{figure}[H]

\centerline{\includegraphics[width=.8\textwidth]{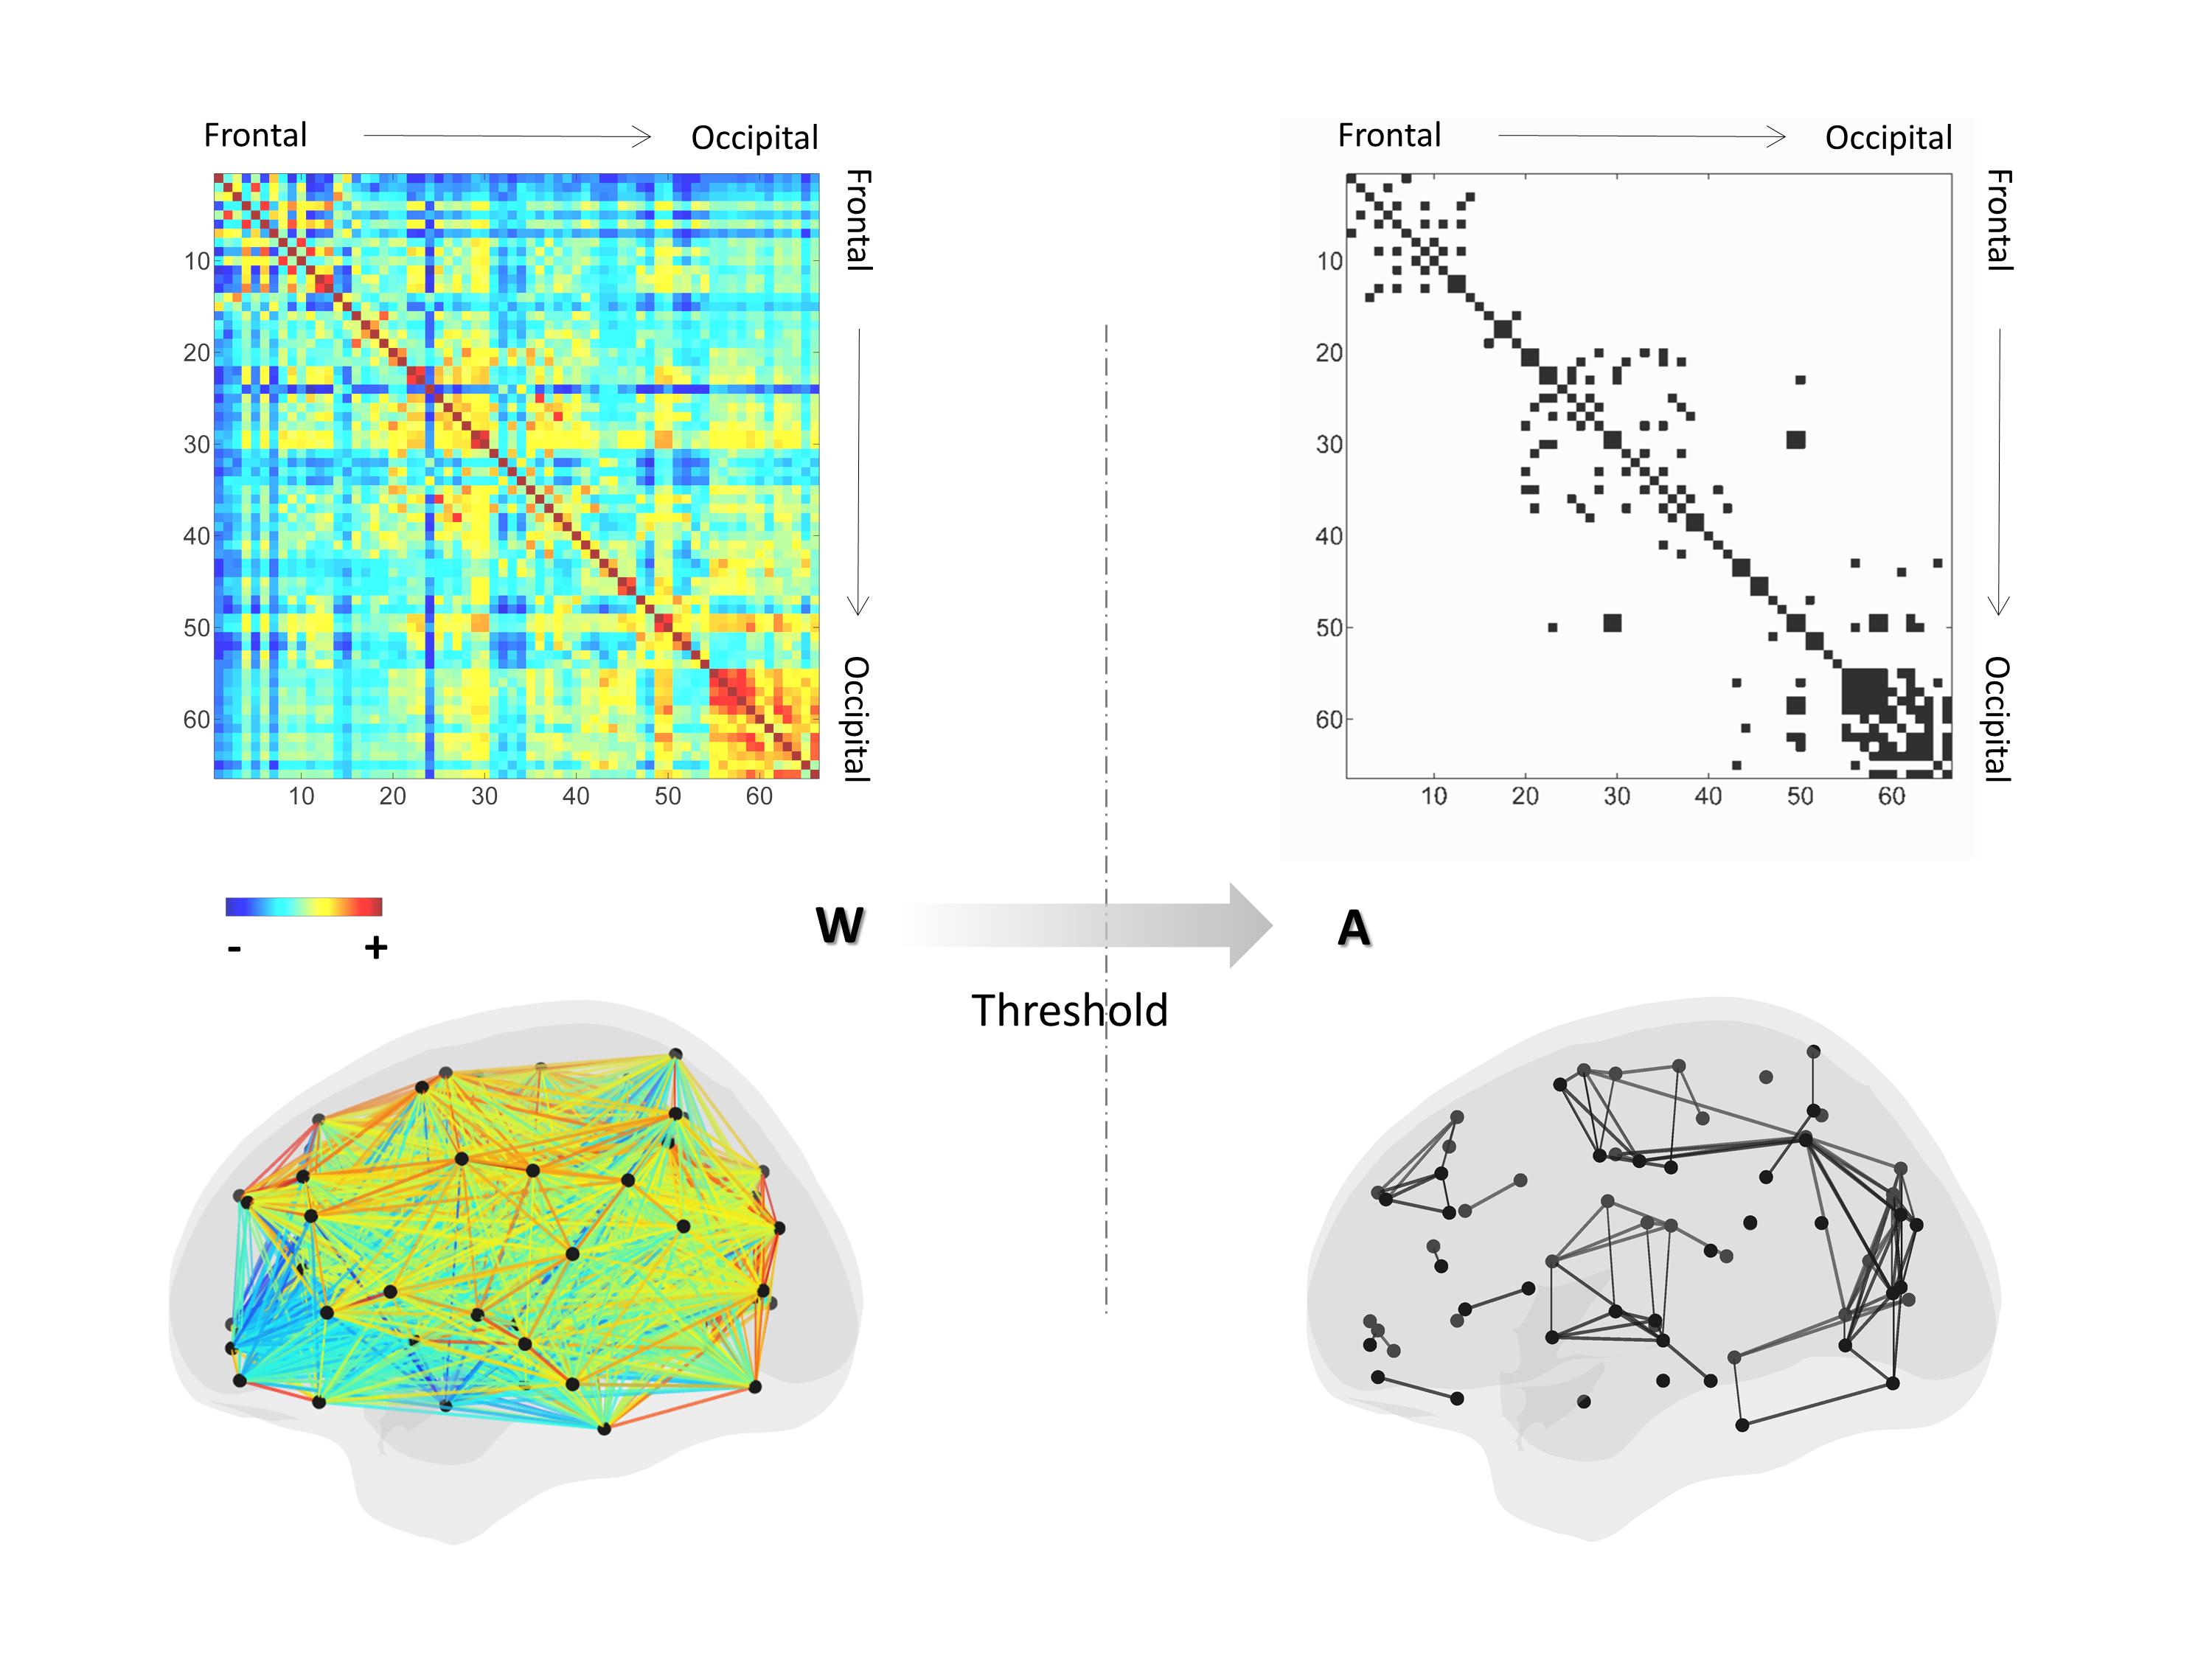}}
\caption{From imaging connectomes to brain networks. As a result of measurements, a raw imaging connectome is mathematically described by full and weighted connectivity matrices $\textbf{W}$. To obtain a sparse brain network, the raw information is filtered and binarized by applying a threshold either on the weights (i.e., the connectivity strength) or on the percentage (i.e., the connection density) of strongest weights to retain in the adjacency matrix $\textbf{A}$.
}\label{fig:SF1}
\end{figure}

\newpage
\begin{figure}[H]

\centerline{\includegraphics[width=1\textwidth]{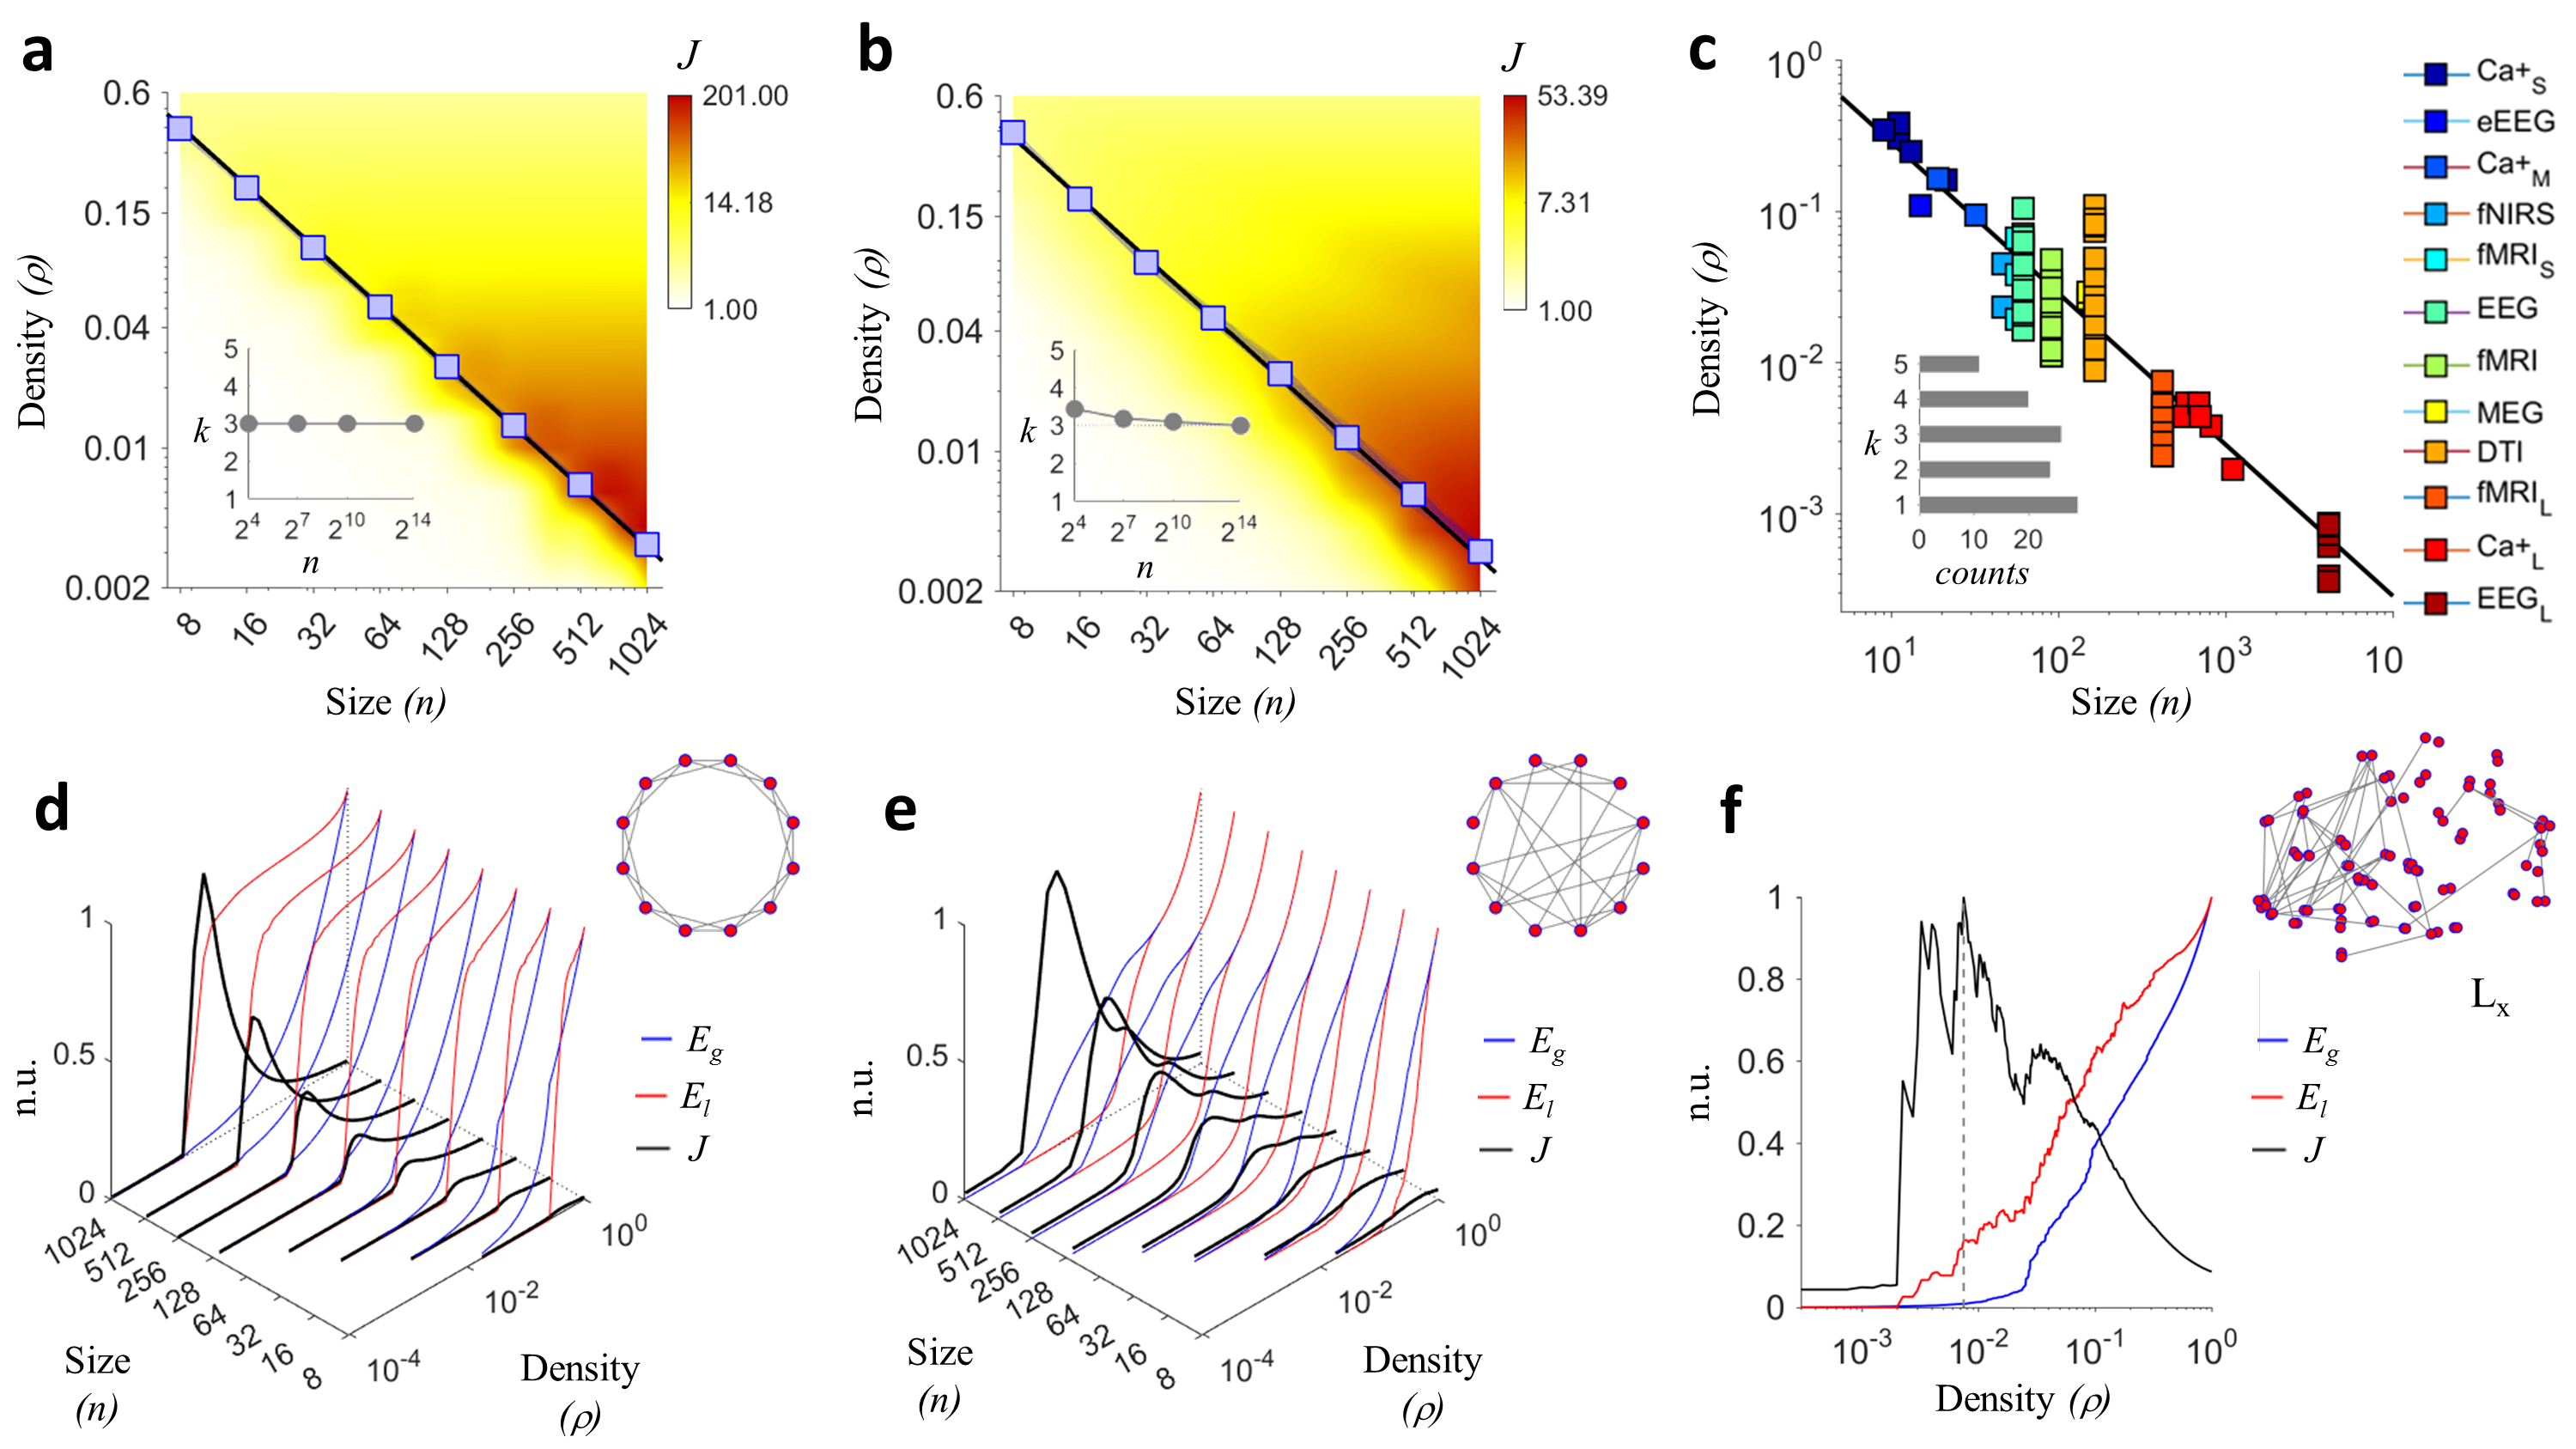}}
\caption{Optimal connection density in synthetic networks and brain networks. 
(\textbf{a}-\textbf{b}) Blue curves show the trends of the optimal density $\rho$ for one-hundred generated lattices and random networks along different sizes $n$. Blue squares spot out the average optimal $\rho$ values. 
The black line shows the fit $\rho=c/(n-1)$ to the data, with $c=3.265$ for lattices and $c=2.966$ for random networks (\textbf{Supplementary Table ~\ref{tab:ST1}}). 
The background color codes for the average value of the quality function $J$. Insets indicate that the optimal average node degree converges to $k=3$ for large network sizes ($n=16834$). 
(\textbf{c}) Optimal density values obtained from individual $J$ profiles for different brain networks. Imaging connectomes come from previously published studies (\textbf{Table ~\ref{tab:1}}). A larger variability can be observed with respect to the values we obtained when considering group-averaged $J$ profiles \textbf{Fig. ~\ref{fig:1}c}. The inset confirms a more uniform distribution for the optimal average node. Nevertheless, the fit $\rho=c/(n-1)$ to the pooled data gives $c=2.87$ (adjusted $R^2=0.946$), which is in practice very close to $k=3$. 
(\textbf{d}-\textbf{e}) Average $J$ profile (black curves) for simulated lattices and random networks as a function of the network size ($n$) and of the density ($\rho$). $J$ values are represented in normalized units (n.u.), having scaled them by the  global maximum obtained for $n=1024$. Blue and red curves show respectively the profiles of the global- ($E_g$) and local-efficiency ($E_l$).
(\textbf{f}) Individual $J$ profile for a representative fMRI connectome (\textbf{Table ~\ref{tab:1}}). The grey dashed line indicates the actual density maximizing $J$, i.e., $\rho=0.008$, corresponding to an average node degree $k=0.712$. This value was very far from the expected optimal $k=3$. Indeed, we noticed that for very low density values the intrinsic brain network structure could not completely emerge and spurious peaks could appear. To improve the quality of the estimate, we averaged the $J$ profiles over the samples in the same group (\textbf{Fig. ~\ref{fig:1}}). The graph illustrates the brain network of a representative healthy subject (lateral view, frontal lobe on the left $L_x$). 
}\label{fig:SF2}
\end{figure}

\newpage
\begin{figure}[H]

\centerline{\includegraphics[width=1\textwidth]{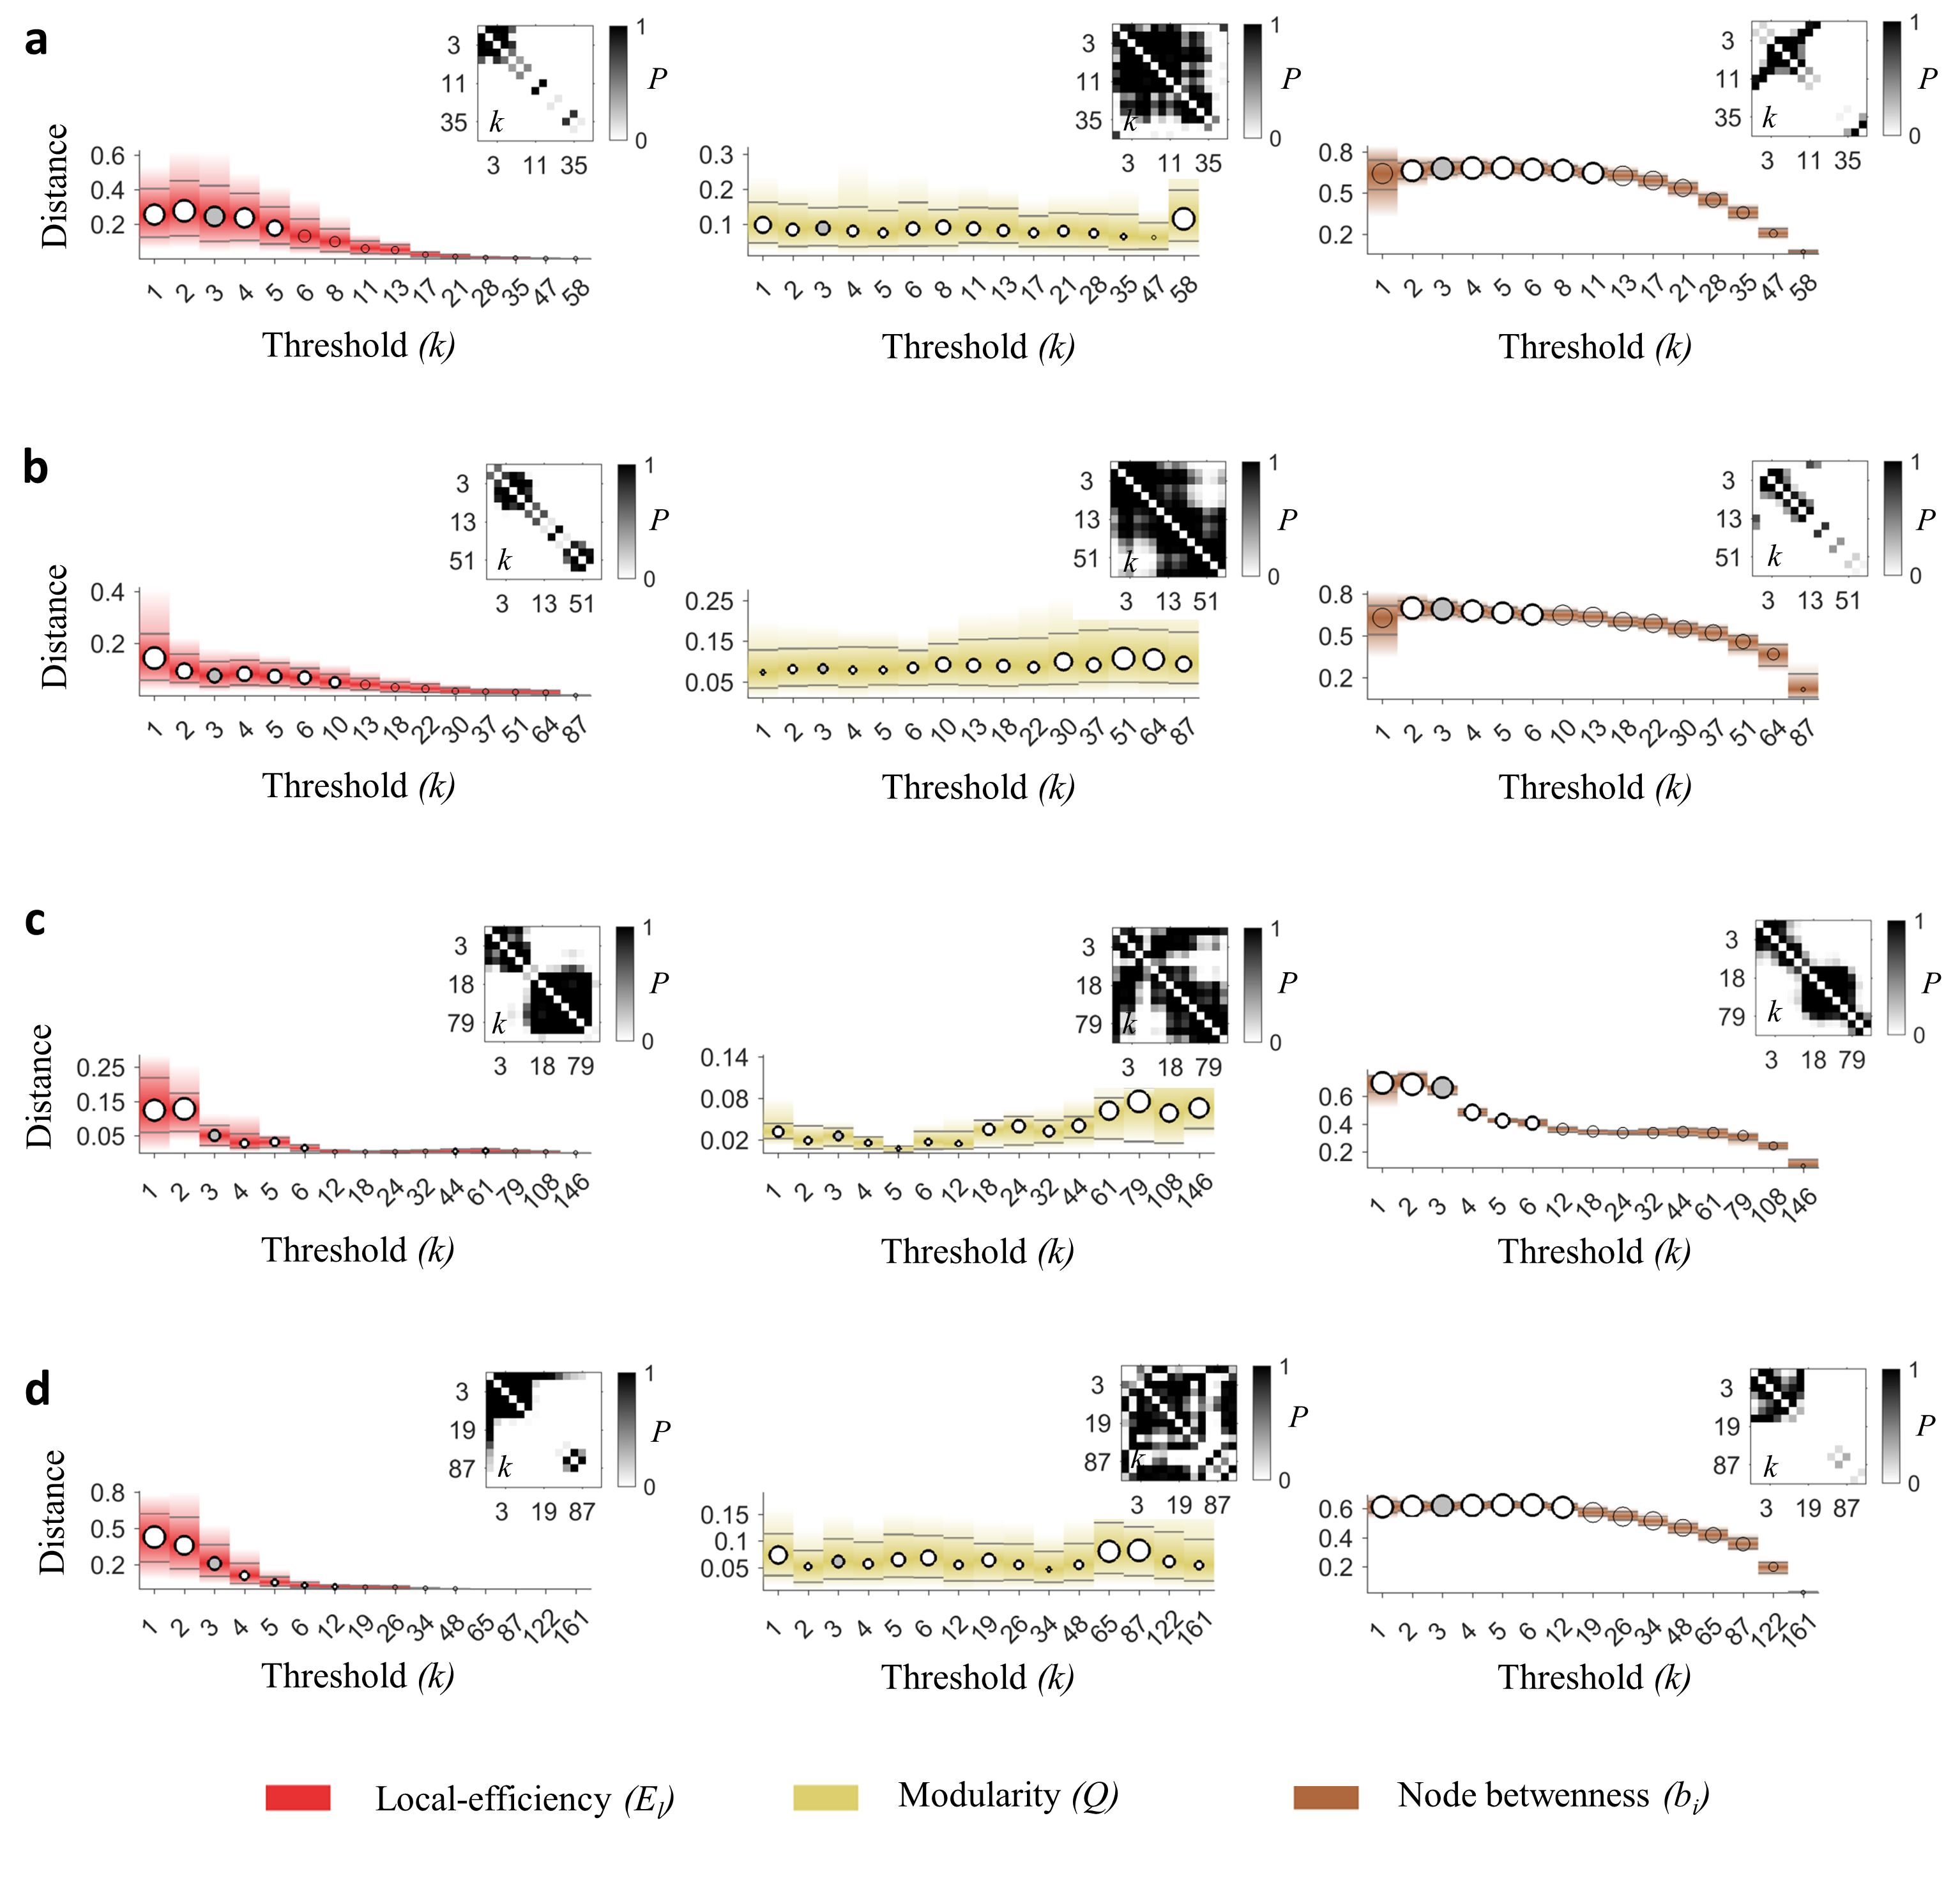}}
\caption{Statistical comparison of brain network distances across different thresholds for local-efficiency $E_l$, modularity $Q$, and node betwenness vector $\textrm{B}=[b_1, ..., b_n]$. Panel (\textbf{a}) show distances for EEG connectomes, (\textbf{b})-fMRI, (\textbf{c})-DTI, (\textbf{d})-MEG. Thresholds are given by the average node degree $k$, which corresponds to a connection density $\rho=k/(n-1)$. Circles correspond to medians; horizontal grey lines correspond to lower and upper quartiles; bar colors shade after quartiles. Overall, the distance significantly depends on the threshold value (Kruskalwallis test, $P < 10^{-54}$; \textbf{Supplementary Table ~\ref{tab:ST2}}). Grey circles represent distances for the optimal threshold $k=3$. White circles denote threshold values for which distances are not significantly different from $k=3$ (Tukey-Kramer post-hoc test, $P\geq0.001$). Transparent circles denote threshold values for which distances are significantly lower  than $k=3$ (Tukey-Kramer post-hoc test, $P<0.001$). Insets show the $P$-values resulting from the Tukey-Kramer post-hoc comparison of distances between all the threshold values.
}\label{fig:SF3}
\end{figure}

\newpage
\begin{figure}[H]

\centerline{\includegraphics[width=1\textwidth]{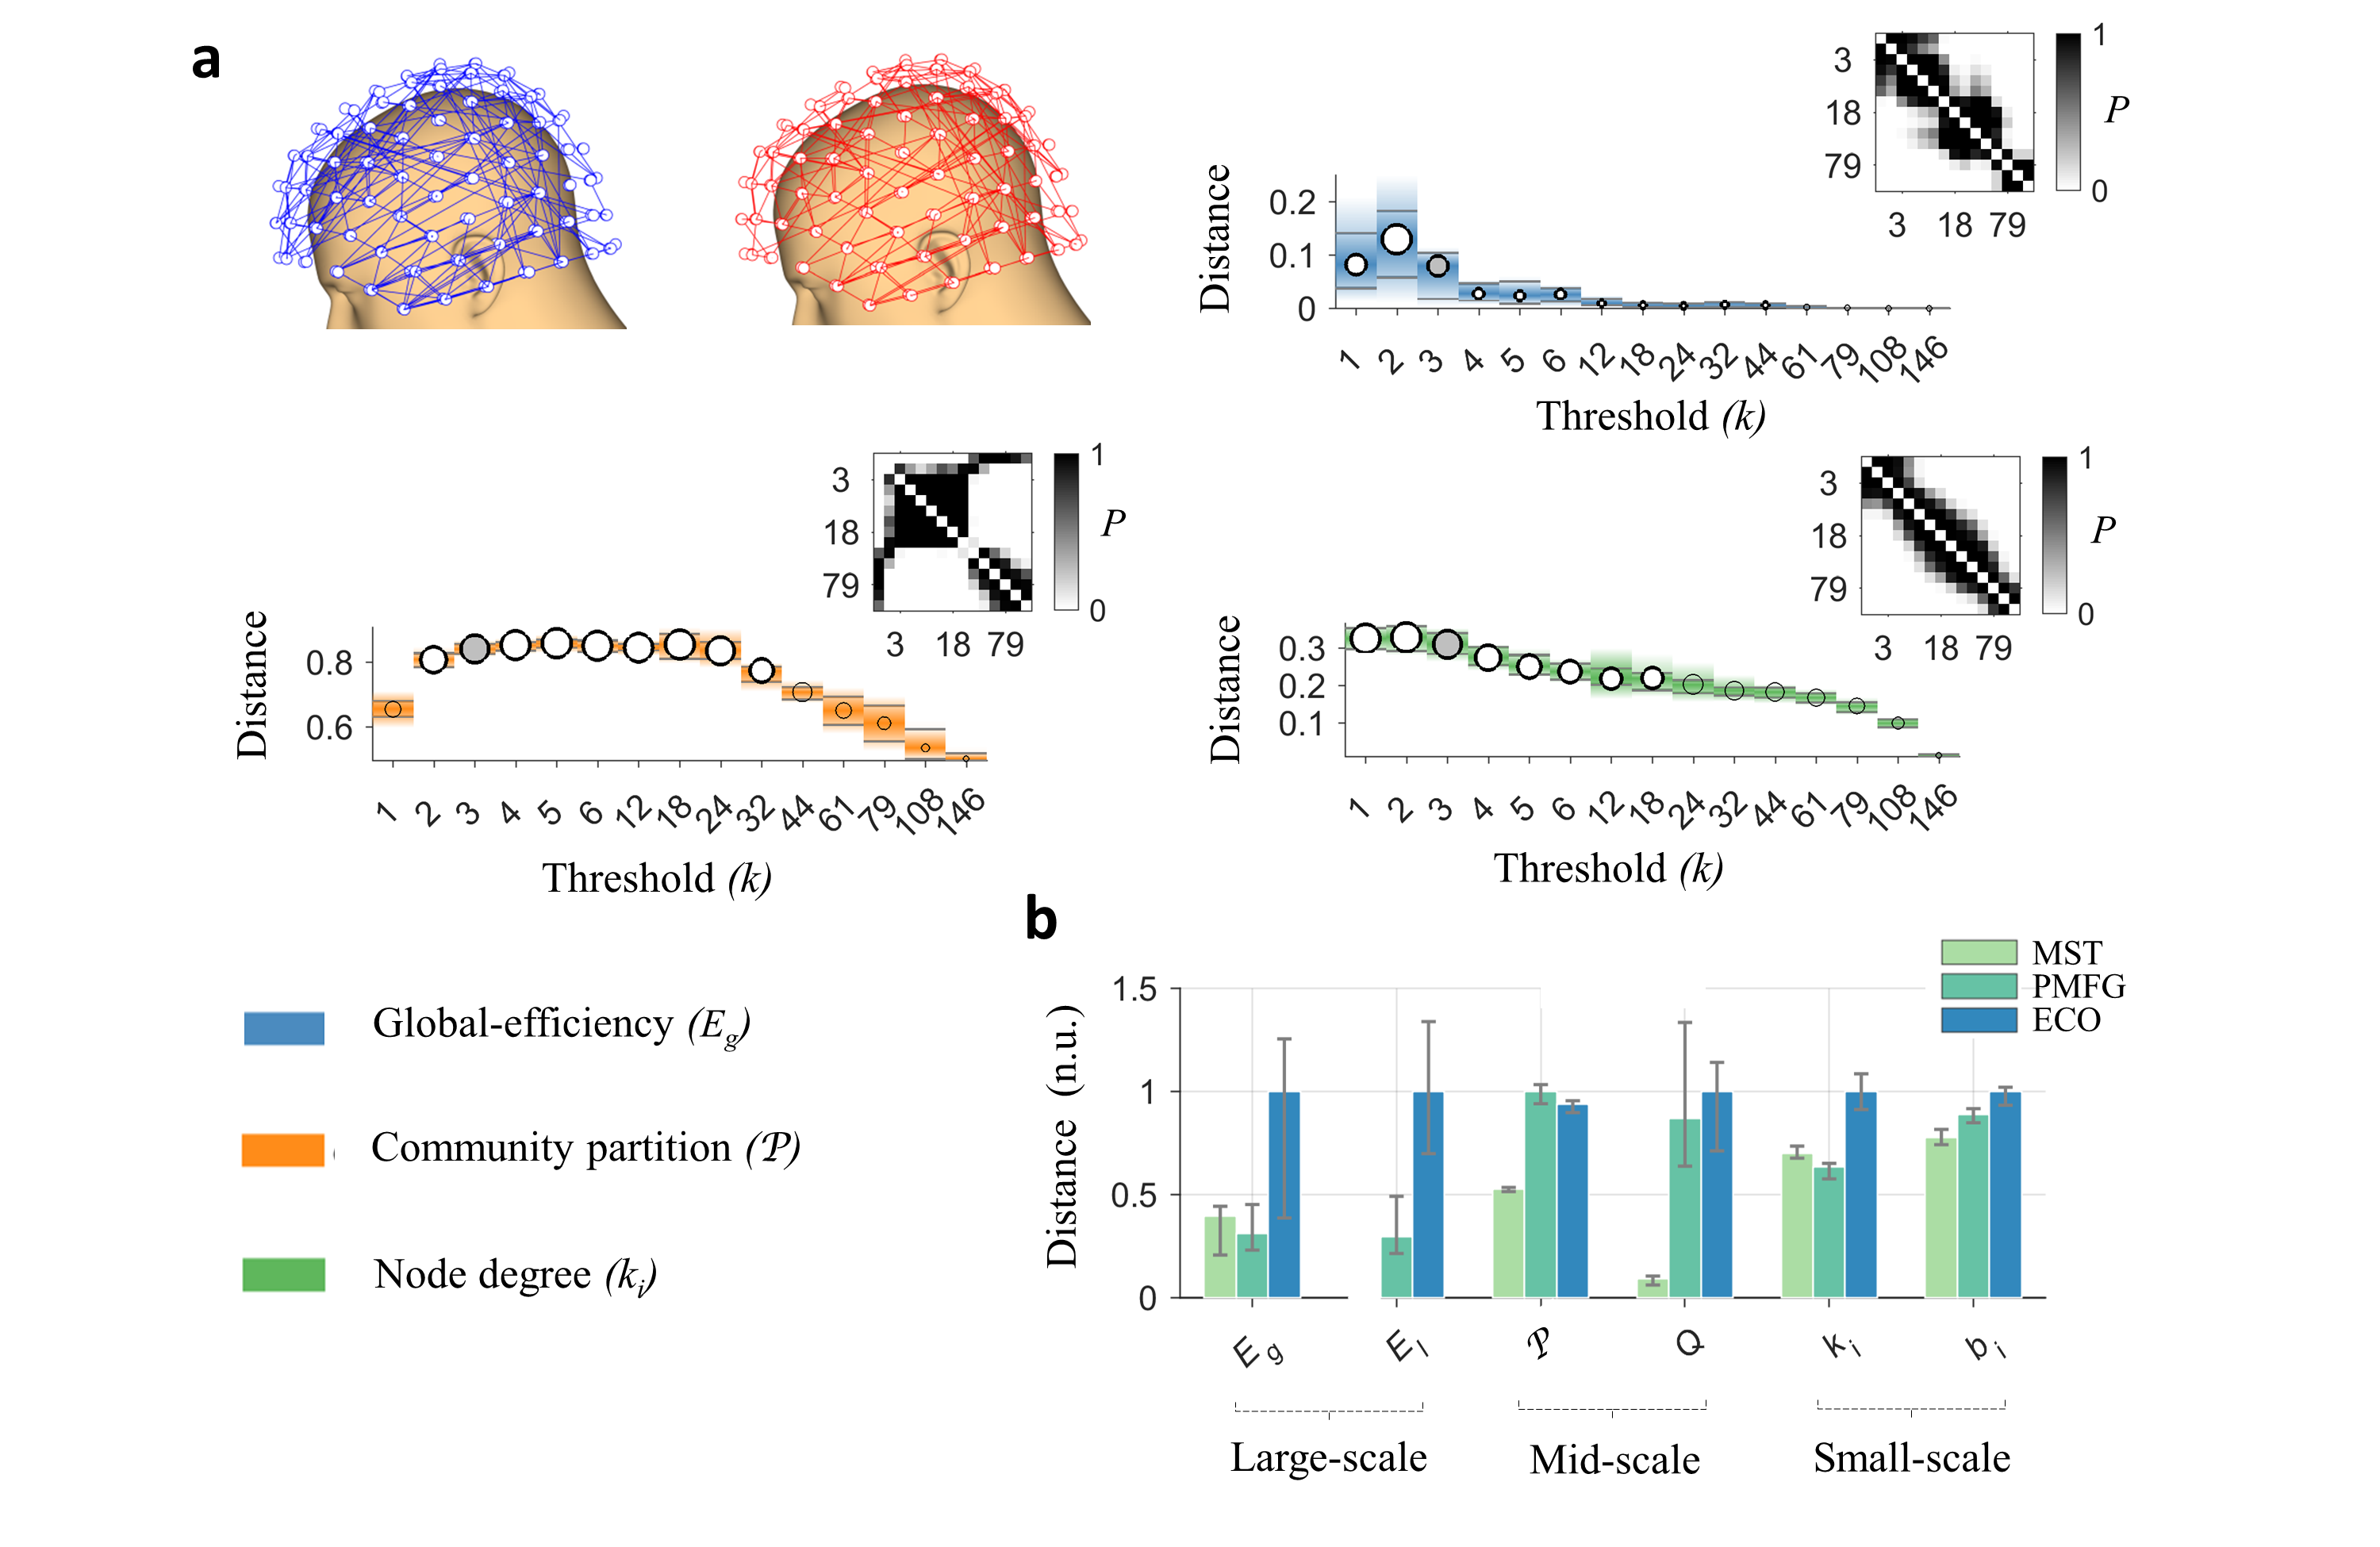}}
\caption{Statistical comparison of brain network distances across thresholds and filtering methods for MEG connectomes.
(\textbf{a}) The top-left panel shows the group-averaged MEG connectomes filtered with ECO for the healthy (blue links) and diseased (red links) (\textbf{Tab. ~\ref{tab:1}}). 
Other panels show brain network distances across different thresholds for global-efficiency $E_g$, community partition $\mathpzc{P}$, and node degree vector $\textrm{K}=[k_1, ..., k_n]$ (Online Method 3). Thresholds are given by the average node degree $k$, which corresponds to a connection density $\rho=k/(n-1)$. Circles correspond to medians; horizontal grey lines correspond to lower and upper quartiles; bar colors shade after quartiles. Overall, the distance significantly depends on the threshold value (Kruskalwallis test, $P < 10^{-15}$; \textbf{Supplementary Table ~\ref{tab:ST3}}). Grey circles represent distances for the optimal threshold $k=3$. White circles denote threshold values for which distances are not significantly different from $k=3$ (Tukey-Kramer post-hoc test, $P\geq0.001$). Transparent circles denote threshold values for which distances are significantly lower than $k=3$ (Tukey-Kramer post-hoc test, $P<0.001$). Insets show the $P$-values resulting from the Tukey-Kramer post-hoc comparison of distances between all the threshold values.
(\textbf{b}) Medians of the distances between brain network properties of samples in the healthy and diseased group for MEG connectomes. Vertical bars denote lower and upper quartiles. Medians and quartiles are normalized for the sake of representation. For all graph quantities ECO gives significantly larger distances as compared to MST (Tukey-Kramer post hoc, $P<0.05$) and, with minor extent, to PMFG (\textbf{Supplementary Table ~\ref{tab:ST4}}). Notably, MST gives null distances for local-efficiency $E_l$ as there are no triangles in tree-like networks. 
}\label{fig:SF4}
\end{figure}

\newpage
\begin{figure}[H]

\centerline{\includegraphics[width=1\textwidth]{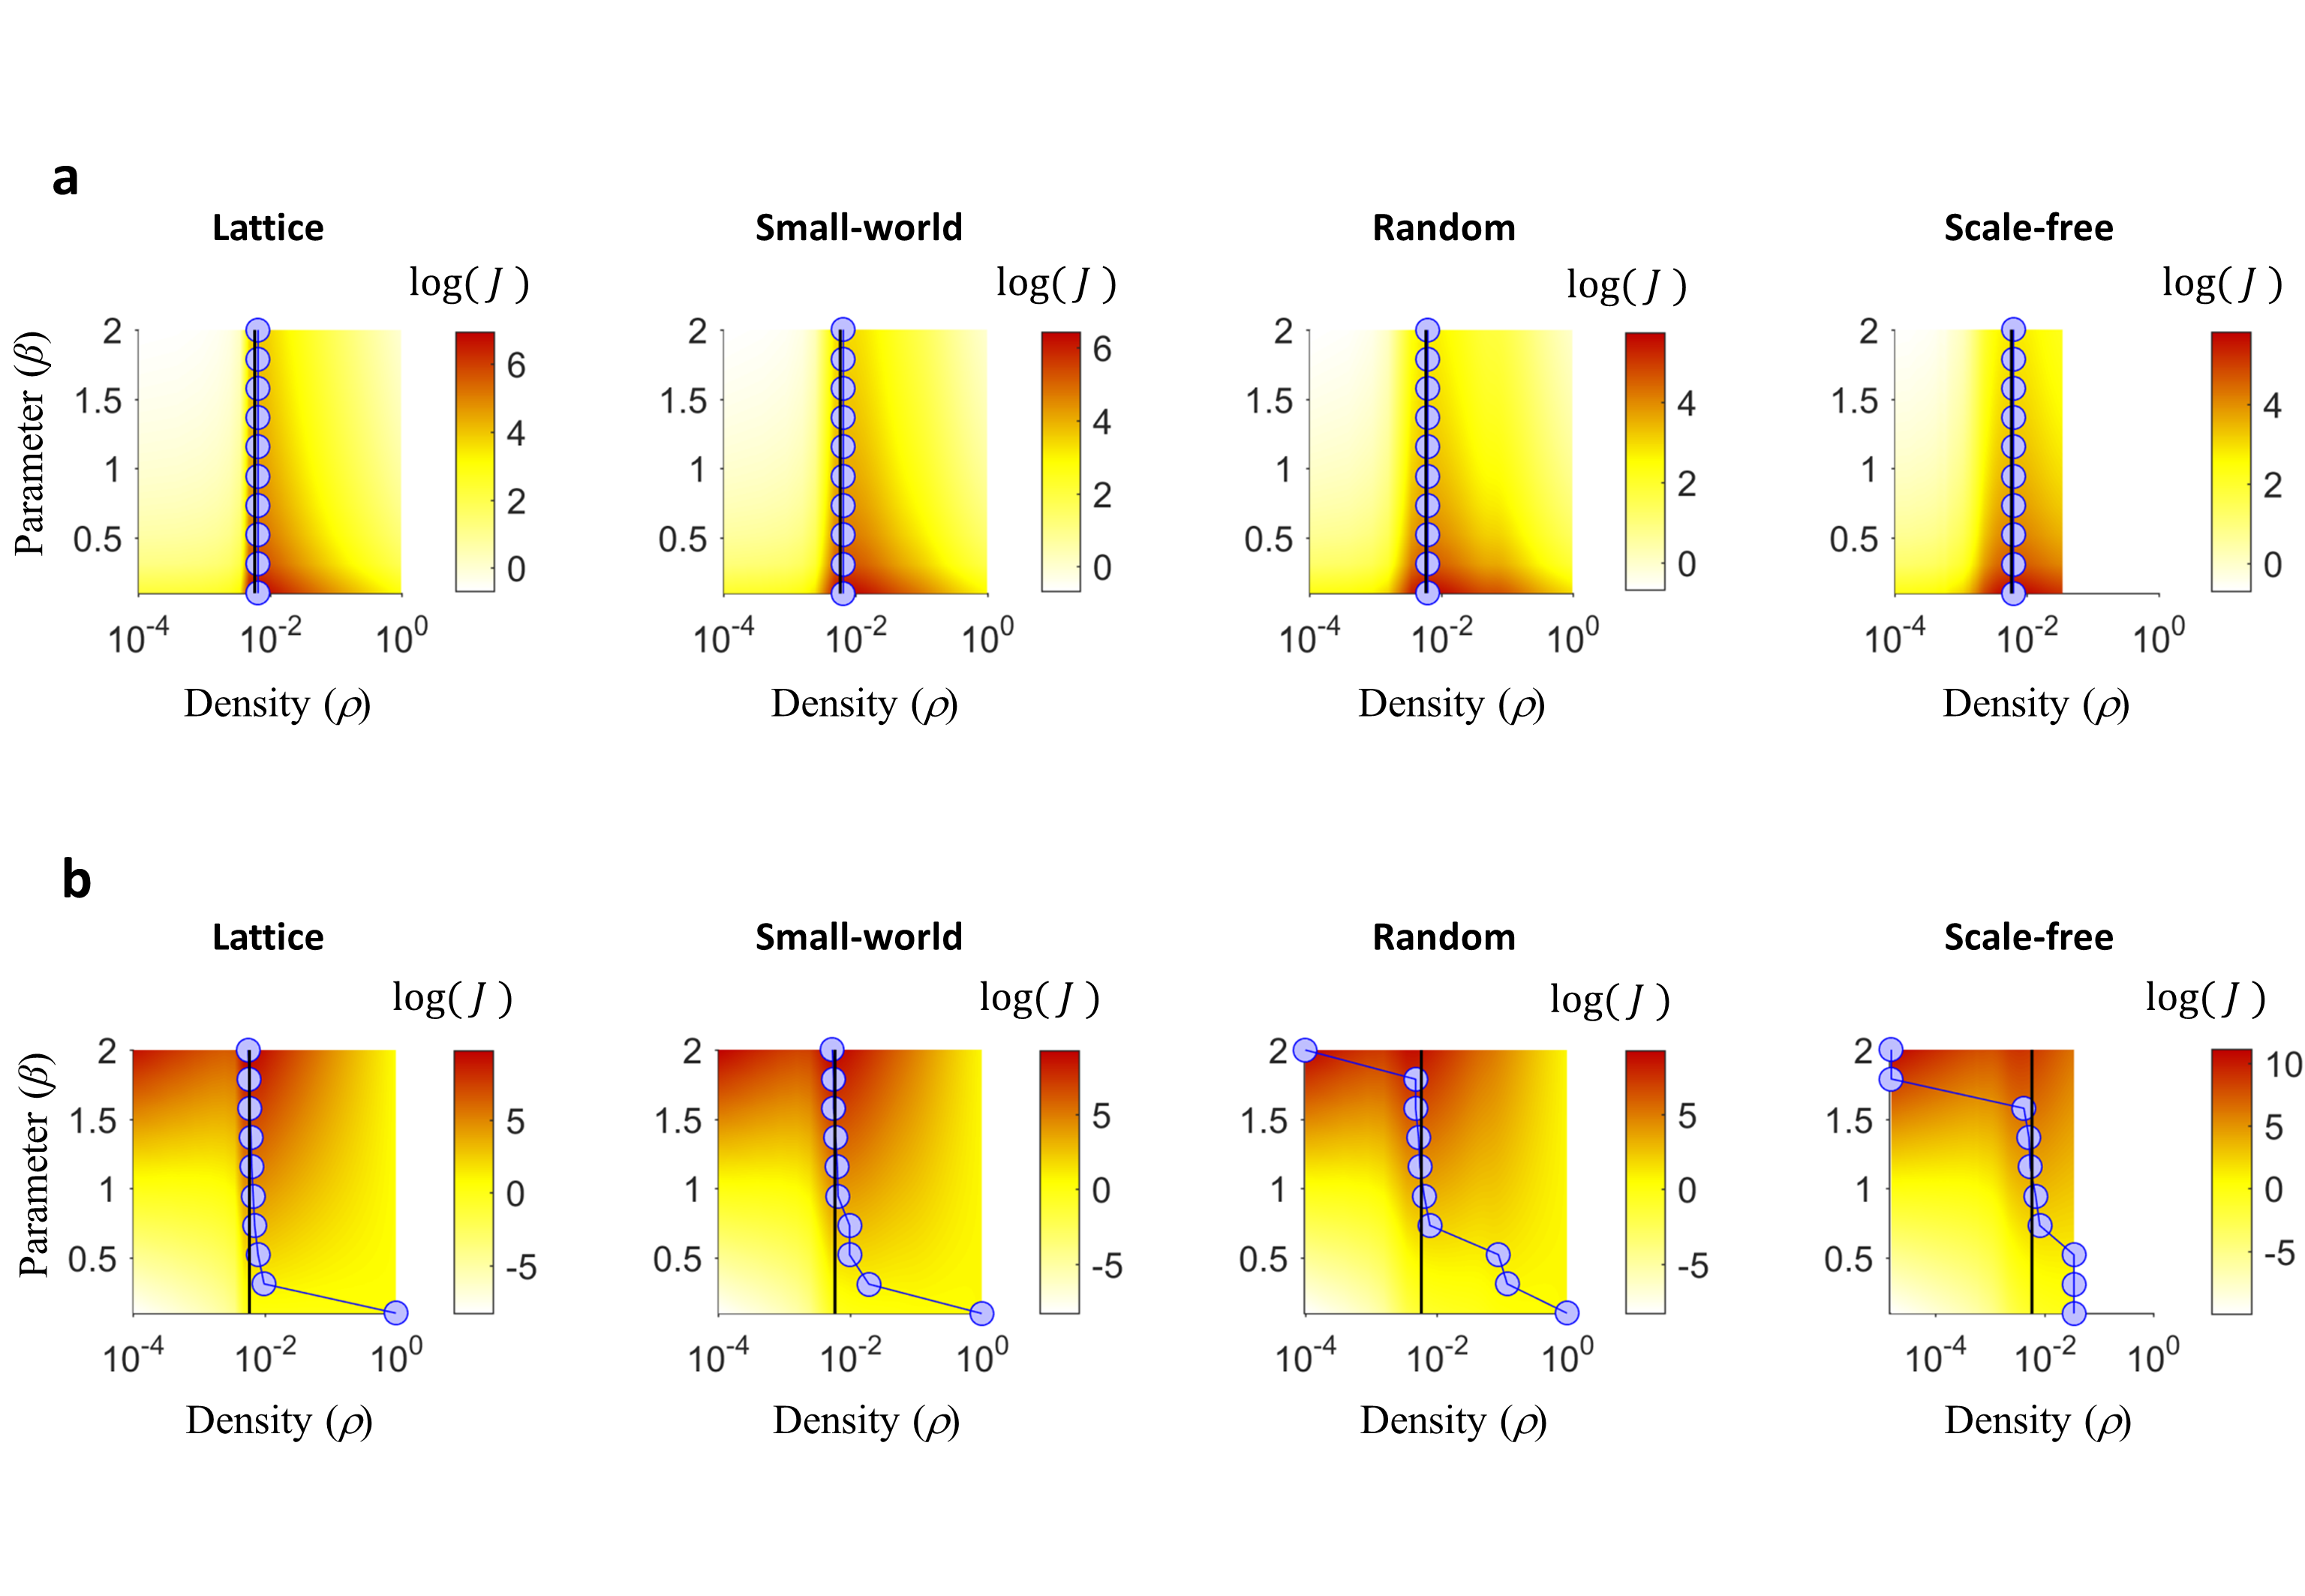}}
\caption{Optimal density obtained with parametric quality functions in syntethic networks. 
Background colors code for the average $J$ values in the logarithmic scale. Blue circles spot out the maximum as a function of the parameter $\beta$ (y-axis). The black line shows the reference optimal density value $\rho=3/(n-1)$ (x-axis).
(\textbf{a}) $J'=\dfrac{E_g+E_l}{\beta\rho}$;
(\textbf{b}) $J''=\dfrac{E_g+E_l}{\rho^\beta}$.
}\label{fig:SF5}
\end{figure}

\newpage
\section*{Supplementary Tables}
\begin{table}[H]

\footnotesize
\centering
\begin{tabular}{c C{2cm} C{2cm} C{2cm} C{2cm}}
 & \textbf{Lattice}  & \textbf{Small-world}  & \textbf{Random}  & \textbf{Scale-free} \\ 
\textit{c} & 3.265 & 3.258 & 2.966 & 3.215 \\  
\textit{R\textsuperscript{2}} & 0.999 & 0.997 & 0.993 & 0.998 
\end{tabular}
\caption{Statistics of data fitting $\rho=c/(n-1)$ for synthetic networks.
The fit's constant $c$ and the adjusted $R^2$ coefficient are reported along different network models.
}\label{tab:ST1}

\end{table}

\newpage
%\begin{figure}[H]
%\renewcommand{\figurename}{Supplementary Table}
\begin{table}[H]

\centerline{\includegraphics[width=1.2\textwidth]{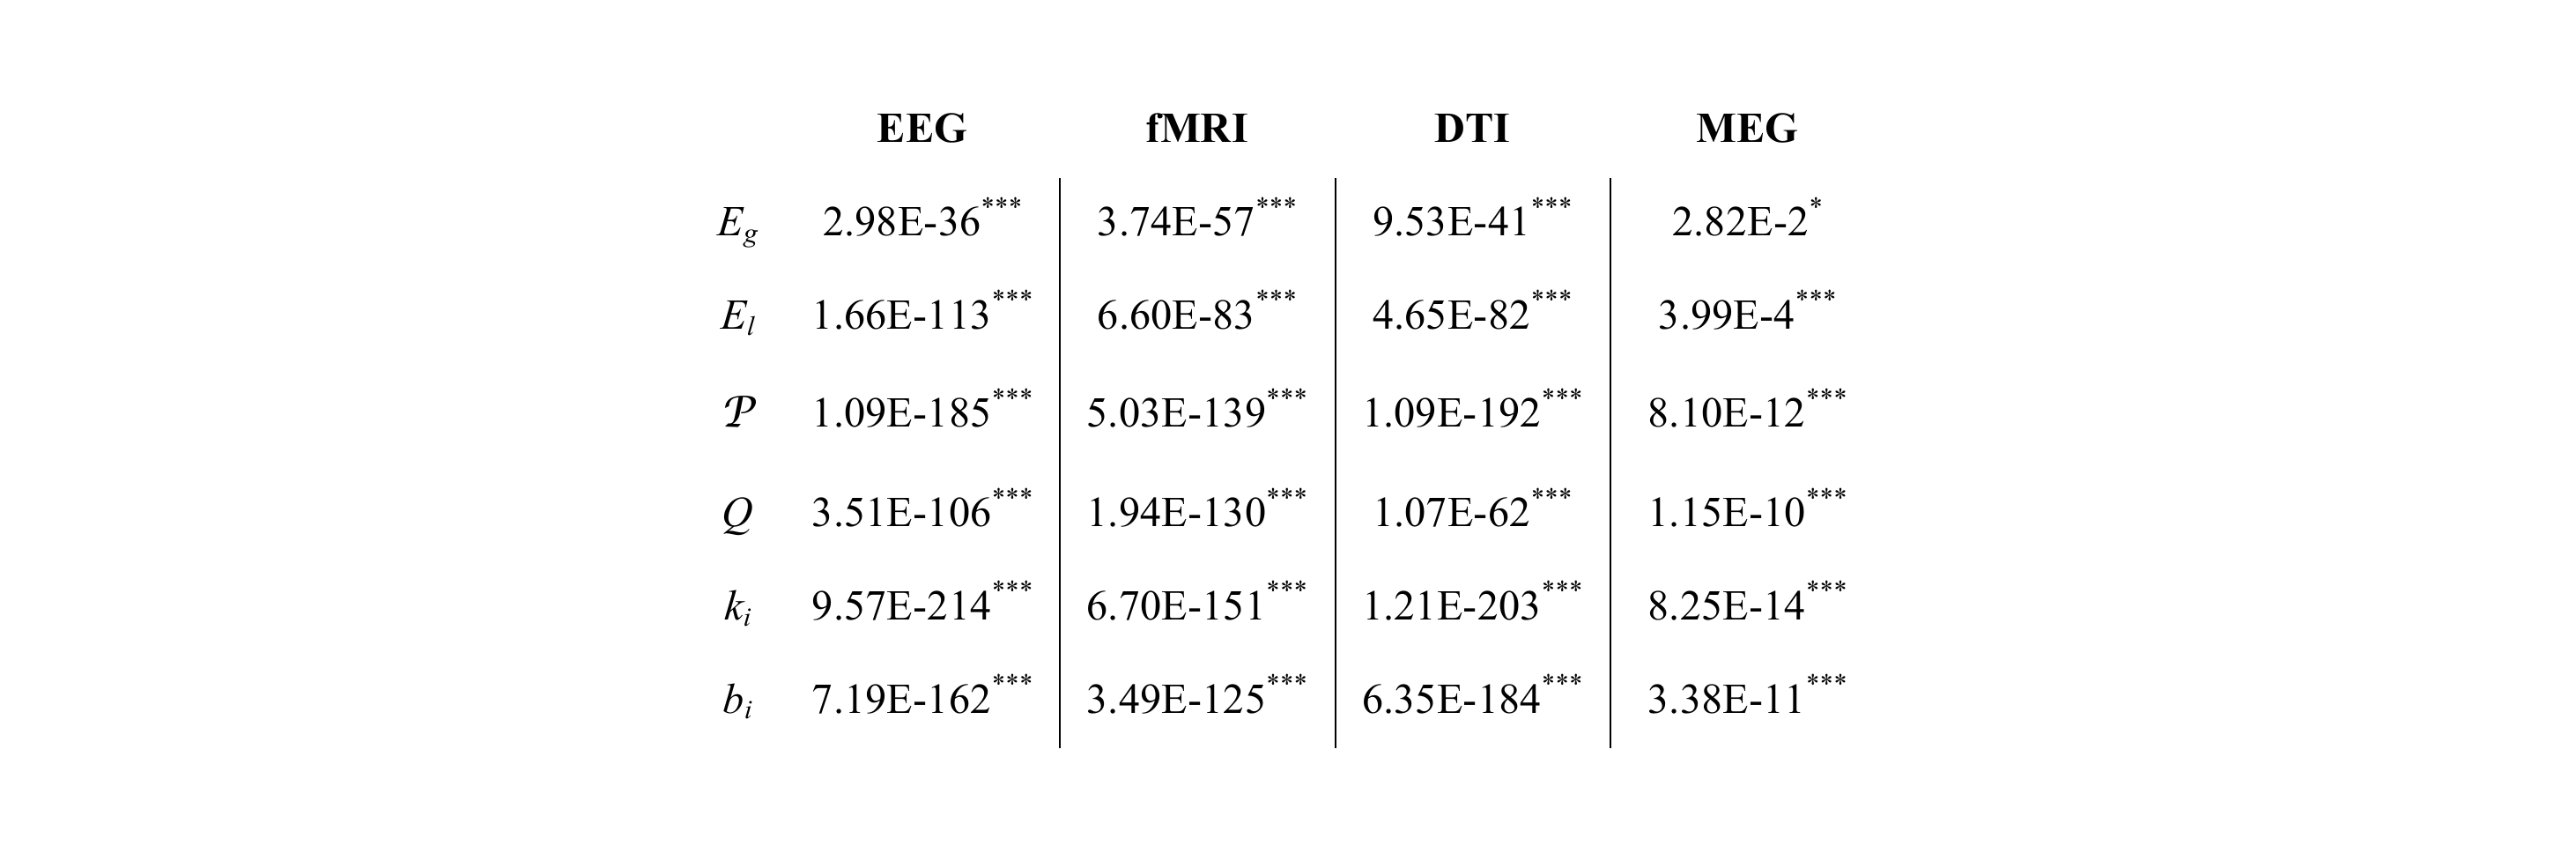}}
\caption{$P$-values from Kruskalwallis tests on brain network distances across different thresholds. Three asterisks denote significant differences with a statistical percentile $P<0.001$; one asterisk corresponds to $P<0.05$.
}
\label{tab:ST2}
\end{table}

\newpage
%\begin{figure}[H]
%\renewcommand{\figurename}{Supplementary Table}
\begin{table}[H]

\centerline{\includegraphics[width=1.2\textwidth]{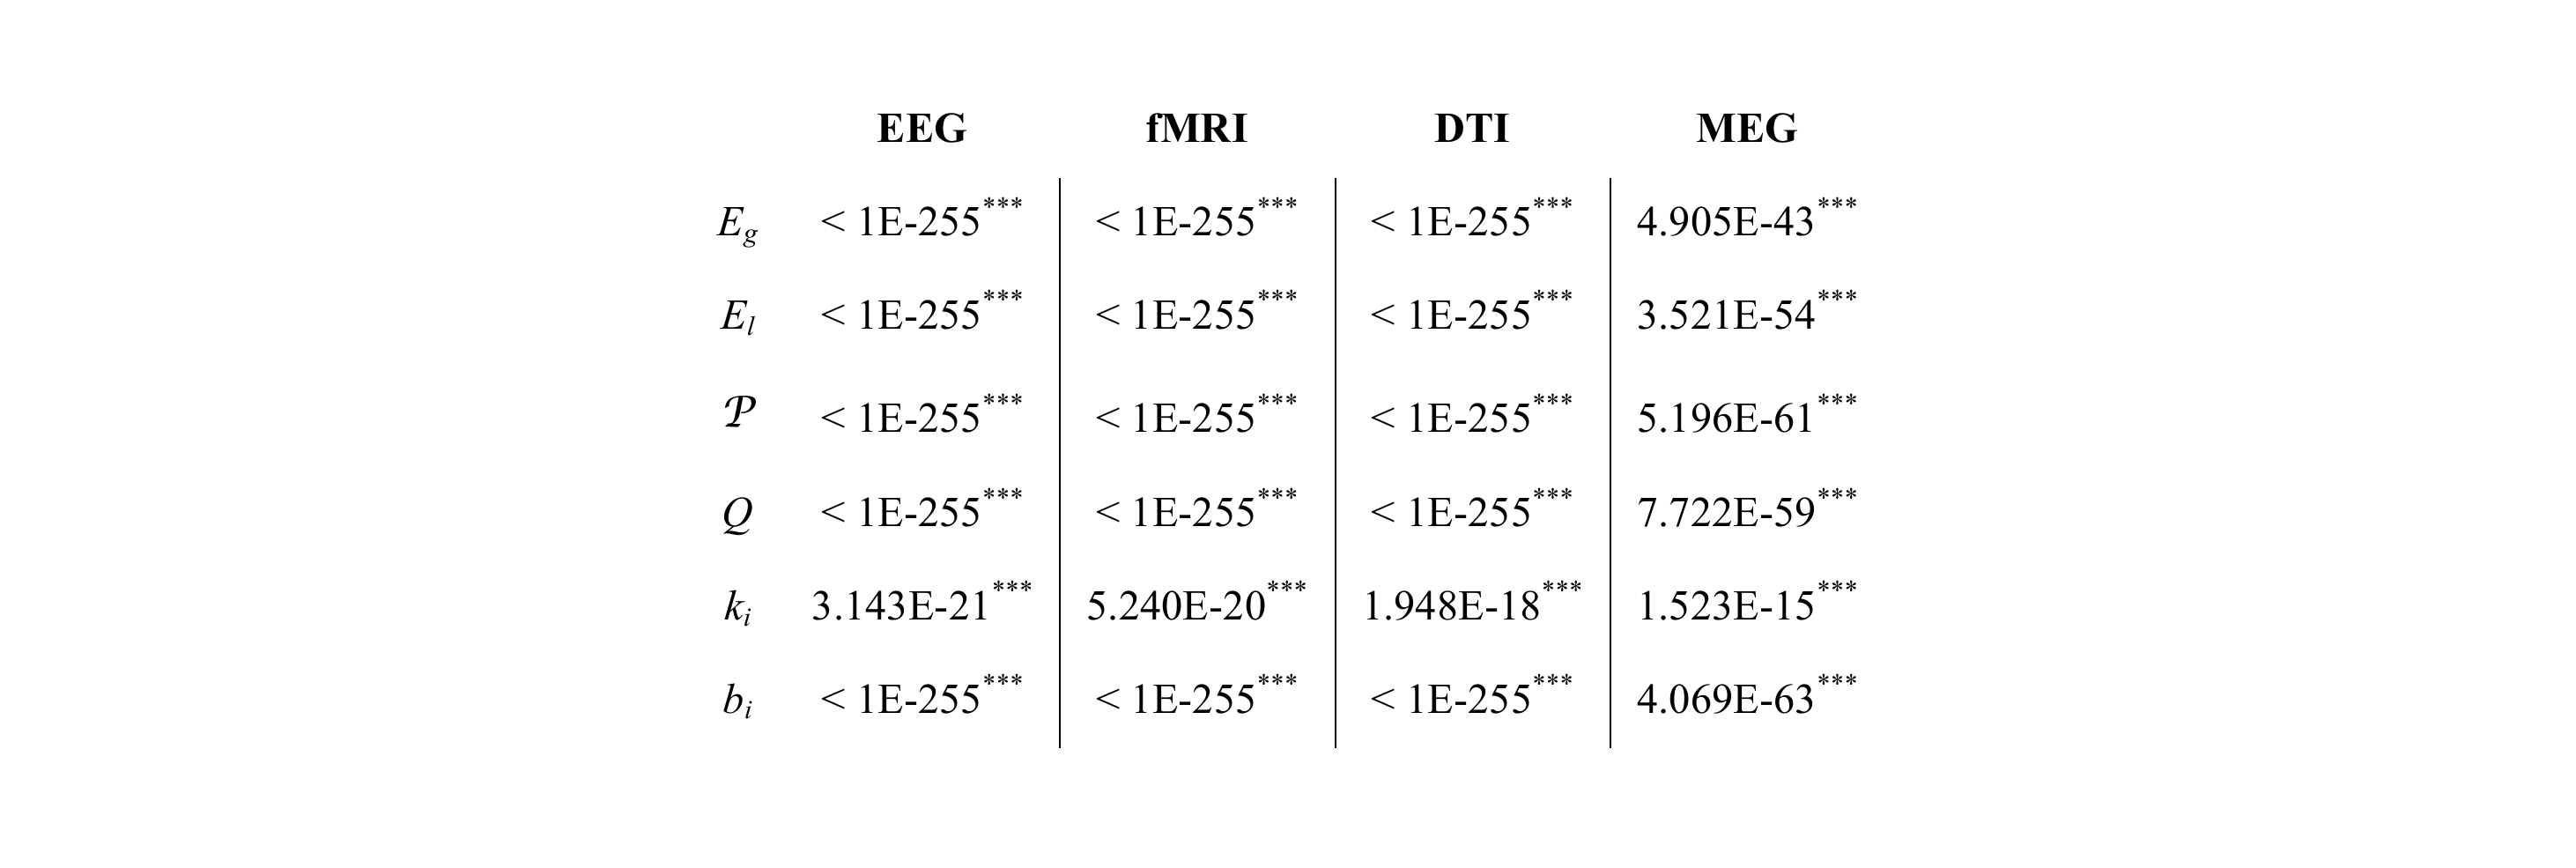}}
\caption{$P$-values from Kruskalwallis tests on brain network distances across different filtering methods. Three asterisks denote significant differences with a statistical percentile $P<0.001$.
}
\label{tab:ST3}
\end{table}

\newpage
%\begin{figure}[H]
%\renewcommand{\figurename}{Supplementary Table}
\begin{table}[H]

\centerline{\includegraphics[width=1.2\textwidth]{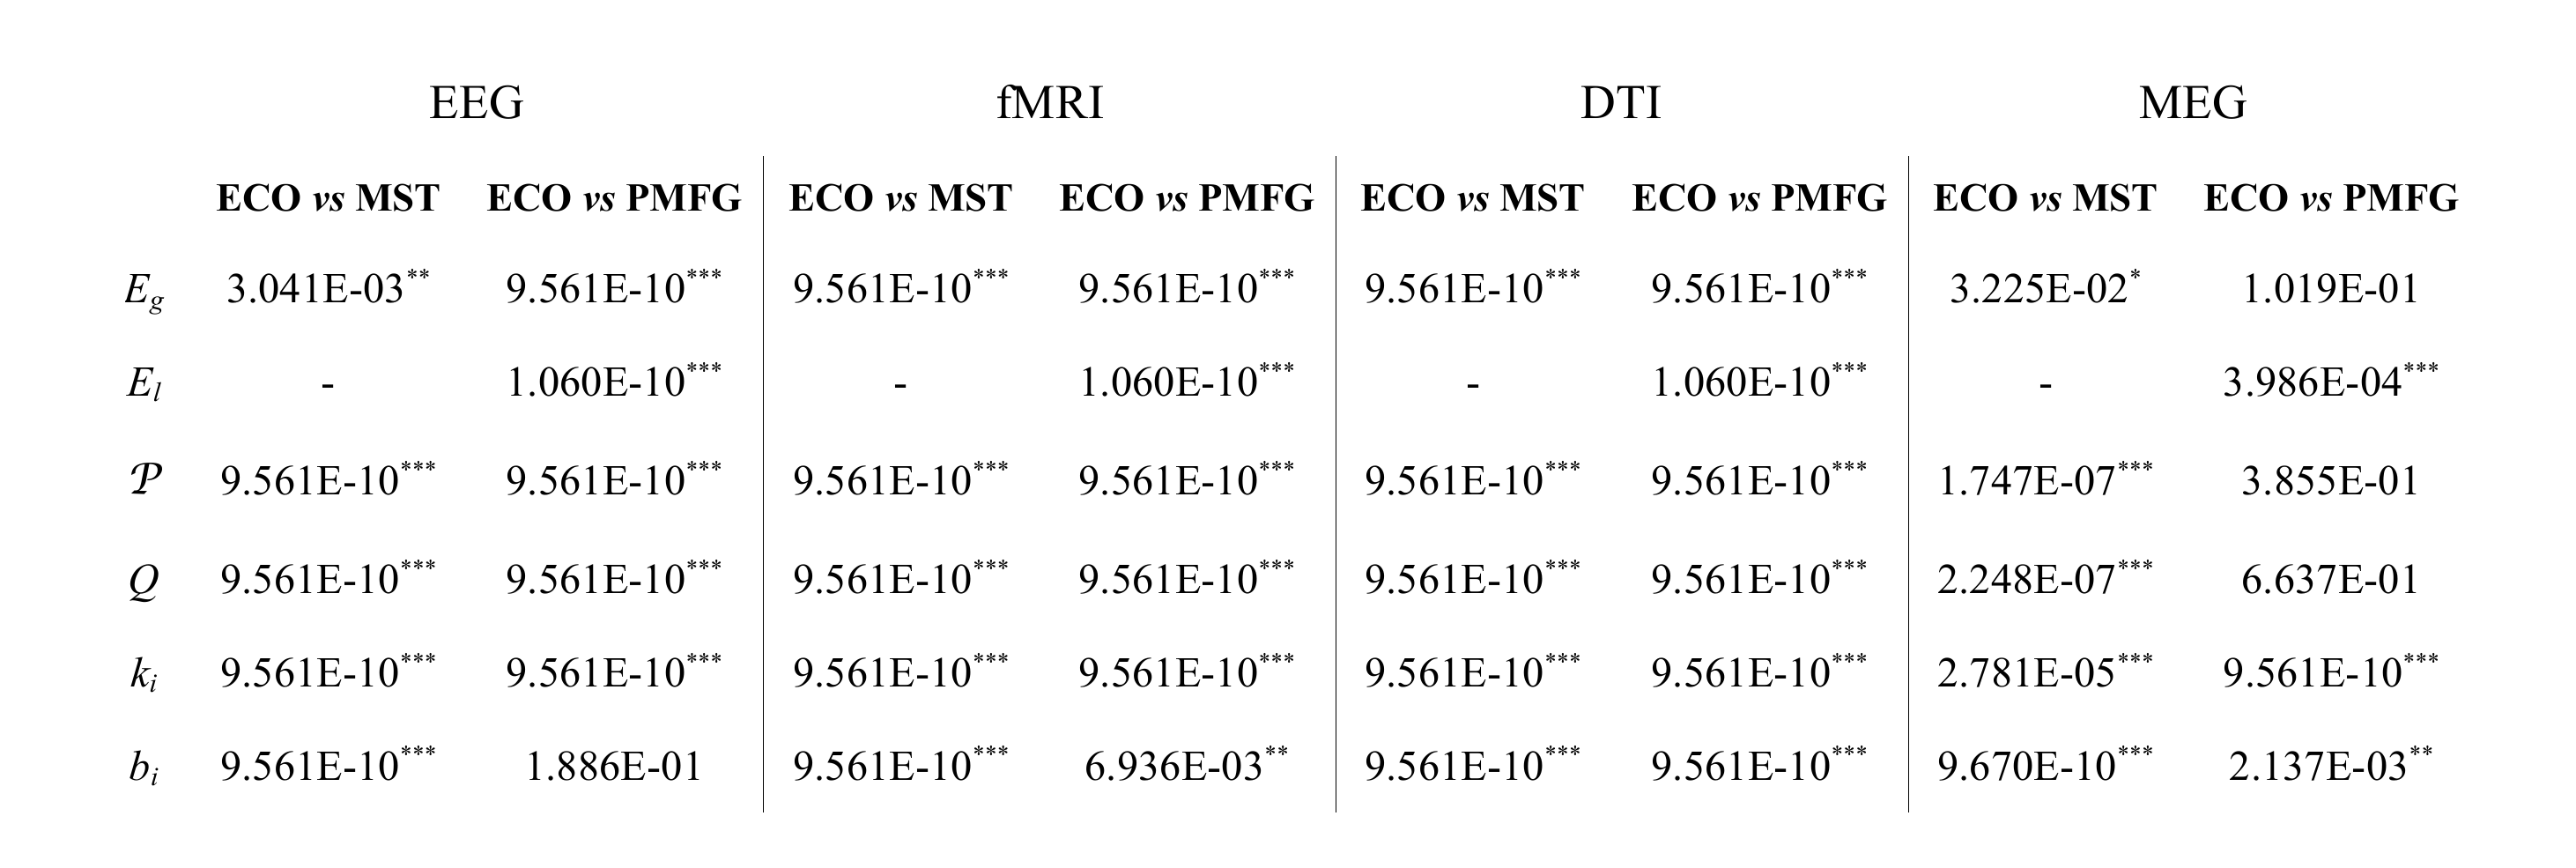}}
\caption{$P$-values from Tukey-Kramer post-hoc tests on brain network distances across different filtering methods. Three asterisks denote significant differences with a statistical percentile $P<0.001$; two asterisks correspond to $P<0.01$, while one asterisk corresponds to $P<0.05$. For local-efficiency ($E_l$), tests were not performed when comparing ECO \textit{vs} MST, as by construction, MST gives null $E_l$ values.
}
\label{tab:ST4}
\end{table}

\newpage
\section*{Supplementary Text}

\subsection*{1. Optimal density in regular lattices and random networks}
Global- $E_{g}$ and local-efficiency $E_{l}$ can be well approximated, respectively, by the inverse of the characteristic path length $L$ and by the clustering coefficient $C$~ \cite{latora_efficient_2001}. We can then rewrite the quality function in Eq. \eqref{eq:1} as $J=(L^{-1}+C)/\rho$. 
In some simple cases, $L$ and $C$ can be expressed as a function of the average node degree $k$ and of the number of nodes $n$ of a network.
 
In particular, for large 1D regular lattices, corresponding to Watts-Strogatz (WS) model with a rewiring probability $p_{ws}=0$, we have $L_0=\dfrac{n}{2k}$ and $C_0=\dfrac{3(k-2)}{4(k-1)}$; while for large random networks ($p_{ws}=1$), we have $L_1=\dfrac{\log{n}}{\log{k}}$ and $C_1=\dfrac{k}{n}$ ~\cite{watts_collective_1998}.
Since the relation $\rho=\dfrac{k}{n-1}$ holds for any network, we can rewrite the quality function $J$ for regular lattices as:

\begin{equation}
J_{0}=2\dfrac{(n-1)}{n} + \dfrac{3(n-1)\rho-6}{4(n-1)\rho^2-4\rho}\label{eq:S1}
\end{equation}
and for random networks:
\begin{equation}
J_{1}=\dfrac{\log{[(n-1)\rho]}}{\rho\log{n}} + \dfrac{(n-1)}{n}\label{eq:S2}
\end{equation}
Notice that the leading contribution to $J$ is coming from $C$ in the case of a lattice and from $L^{-1}$ in the case of a random network. 

For these synthetic networks we can determine analytically the optimal value of $\rho$ that maximizes the quality function $J$. 
In particular, by deriving with respect to $\rho$ and equating to zero, we obtained for lattices the following solution which satisfies the requirement of connectedness ($\rho\geq 2/n$): 
\begin{equation}
\rho_{0}=\dfrac{2+\sqrt{2}}{n-1}\label{eq:S3}
% \quad k_{0}=2+\sqrt{2},  \quad J_{0}=\dfrac{2(n-1)}{n} + \dfrac{3\sqrt{2}(n-1)}{4(4+3\sqrt{2})} \simeq 0.13n 
\end{equation}
As for random networks we obtained:
\begin{equation}
\rho_{1} = \dfrac{e}{n-1}\label{eq:S4}
%, \quad k_{1}=e, \quad J_{1}=\dfrac{(n-1)}{n} + \dfrac{(n-1)}{e\log{n}} \simeq \dfrac{(n-1)}{e\log{n}} 
\end{equation}
It follows from Eq. \eqref{eq:S3} and Eq. \eqref{eq:S4} that in both cases the optimal density can be written as $k/(n-1)$, where the constant (i.e., the average node degree) is approximately equal to $3$.
Without loss of generality we referred here to undirected networks. For directed networks the same results hold, $k$ corresponding to the average node in/out-degree.

\newpage
\subsection*{2. Optimal density in alternative quality functions}

We considered alternative quality functions combining $E_g$, $E_l$ and $\rho$. 
For each new $J$, we checked analytically the existence of an optimal density in both regular lattices and random networks.
We excluded the quality functions for which we obtained indefinite, non-closed or trivial solutions.

\begin{itemize}
\item $J=E_g+E_l-\rho = 1/L + C - \rho$

By substituting the expression of $L$ and $C$ for random networks we obtain:
\begin{equation}
J_{1}=\dfrac{\log{k}}{\log{n}} + \dfrac{k}{n} - \dfrac{k}{n-1}\label{eq:S8}
\end{equation}

For the sake of simplicity we solved with respect to $k$, knowing that $\rho=k/(n-1)$. When derivating and equating to zero we had $k=\dfrac{n(n-1)}{\log{n}}$, which leads to the impossible condition $\rho=n/\log{n}>1$.

\item $J=E_g - \rho = 1/L - \rho$

By using the expression of $L$ for lattices we obtain:
%ca
\begin{equation}
J_{0}=\rho \left( 2\dfrac{(n-1)}{n} -1 \right) \label{eq:S9}
\end{equation}

When derivating and equating to zero we had $n=2$ and we cannot solve with respect to $\rho$.

\item $J=E_l-\rho = C -\rho$

By substituting the expression of $C$ for random networks we obtain:
\begin{equation}
J_{1}=\dfrac{k}{n} - \dfrac{k}{n-1}\label{eq:S10}
\end{equation}

When derivating and equating to zero we had $1/n=1/(n-1)$ and we could not solve with respect to $\rho$.

\item $J=E_gE_l/\rho = (C/L)/\rho$

By substituting the expression of $L$ and $C$ for random networks we obtain:
\begin{equation}
J_{1}=\dfrac{n-1}{n \log{n}} \log{k}\label{eq:S11}
\end{equation}

When derivating and equating to zero we had the trivial solution $k=0$.

\end{itemize}

Similarly, it is easy to prove that neither $J=E_g/\rho$ nor $J=E_l/\rho$ admitted meaningful solutions in lattices or random networks.

\newpage
\subsection*{3. Optimal density in parametric quality functions}

We introduced a parameter $\beta$ to tune the contribution of the connection density in $J$.
In particular, we evaluated two quality functions:
\begin{equation}
J'=\dfrac{E_g+E_l}{\beta\rho}\label{eq:S7}
\end{equation}
and
\begin{equation}
J''=\dfrac{E_g+E_l}{\rho^\beta}\label{eq:S8}
\end{equation}
where we fixed $\beta \in[0, 2]$. In both cases, we obtained the original expression of $J$ when $\beta=1$.
We evaluated the above quality functions over one-hundred synthetic networks generated according to Online method 2. 
For the sake of simplicity we only considered networks with size $n=512$.
Results show that for $J'$ the parameter $\beta$ has no effect on the optimal density, which is always $\rho=3/(n-1)$ \textbf{Supplementary Fig. ~\ref{fig:SF5}a}.
As for $J''$, the optimal density can change when we move far from $\beta=1$ \textbf{Supplementary Fig. ~\ref{fig:SF5}b}. This is particularly true for both random networks and scale-free networks.
 
 %\bibliography{Mybib_20032016}
 
%\end{document}
